# Supplementary material for: Sparse Depth Sensing for Resource-Constrained Robots
Source: arXiv:1703.01398 source file (2017-10-15)
Supplement: Supplementary file 1 [file figureAppendix.tex]

\begin{figure}[h]
\begin{minipage}{\textwidth}
\begin{tabular}{cc}\begin{minipage}{4cm}\centering\includegraphics[height=3cm]{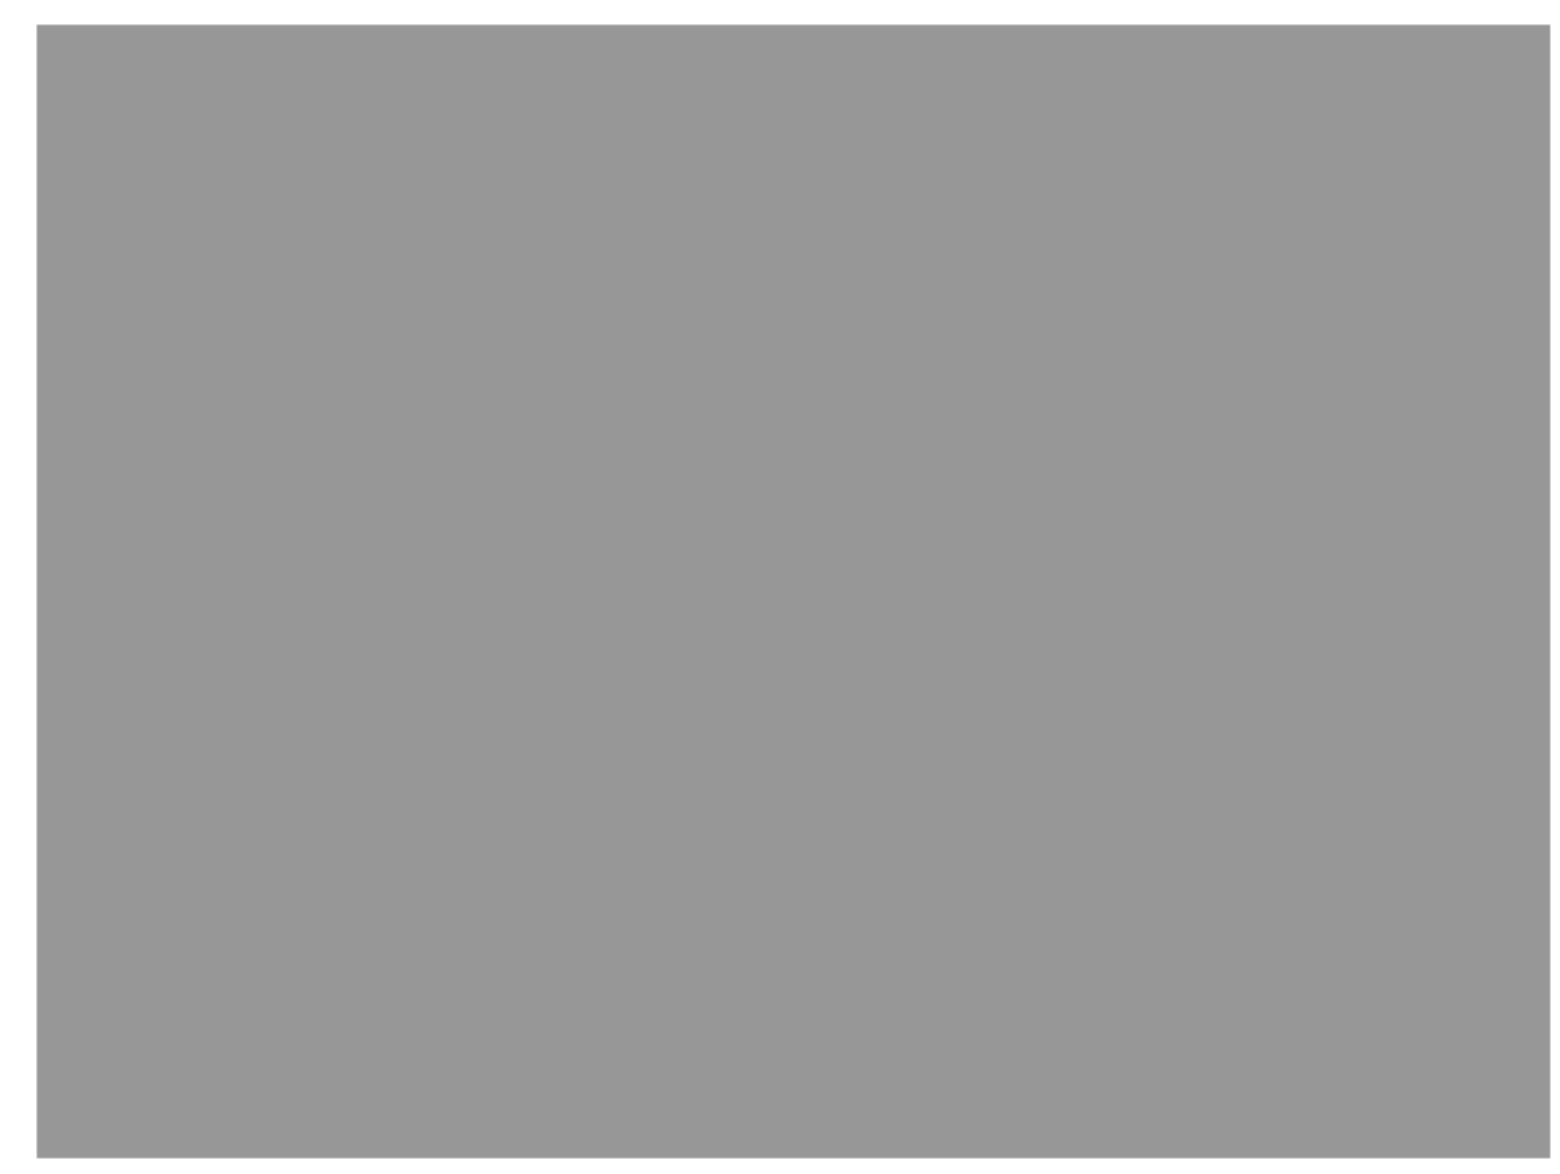} 
\end{minipage}
&  \;\;
\begin{minipage}{4cm}\centering\includegraphics[height=3cm]{gray} 
\end{minipage}
\\
\begin{minipage}{4cm}\centering\includegraphics[height=3cm]{gray} 
\end{minipage}
&  \;\;
\begin{minipage}{4cm}\centering\includegraphics[height=3cm]{gray} 
\end{minipage}
\\
\begin{minipage}{4cm}\centering\includegraphics[height=3cm]{gray} 
\end{minipage}
&  \;\;
\begin{minipage}{4cm}\centering\includegraphics[height=3cm]{gray} 
\end{minipage}
\end{tabular}
\end{minipage}\caption{
Gazebo results (uniform sampling, l1 versus naive)
(a) Error for increasing number of samples on the edges
(b) Error for increasing number of measurements on entire image
(c) Error for increasing noise (measurements uniform in edges)
(d) Error for increasing noise (measurements uniform in image)
\green{ZED results (uniform sampling, l1 versus naive)
(e) Error for increasing number of samples on the edges.
(f) Error for increasing number of measurements on entire image.}
\vspace{-0.5cm}
}
\label{fig:recovery2D}
\end{figure}
